# Supplementary material for: Pre-trained Trojan Attacks for Visual Recognition
Source: arXiv:2312.15172 source file (2023-12-23)
Supplement: Supplementary file 1 [file appendix.tex]

\appendix
\counterwithin{table}{section}
\counterwithin{figure}{section}
\section*{Appendix}
\section{Implementation Details}

\textbf{Tasks and Datasets.} 

\emph{ImageNet}. This dataset is a large-scale visual database for different computer vision tasks. It consists of 1,000 class labels, which contain 1,281,167 training images and 50,000 validation images. It also provides bounding box labels that can be used for object detection, where the training/validation set contains 543,922 and 50,000 images.

\emph{COCO}. This dataset consists of 80 categories of objects and offers comprehensive annotation information, including bounding boxes, instance segmentation masks, and key points. The training set comprises 118,287 images, and the validation set contains 5,000 images.

\textbf{Backdoor Attacks.} 

\emph{BadNets} \cite{gu2019badnets}. It adds a fixed white pattern to the bottom right corner of the clean image.

\emph{Blended} \cite{chen2017targeted}. This method blends a fixed universal image as the trigger with a clean image. We set its opacity to 20\%.

\emph{SIG} \cite{tran2018spectral}. It adds sinusoidal signal perturbations as the trigger on the clean image. We specify the perturbation strength as 40 and the frequency parameter as 6.

\emph{SSBA} \cite{li2021invisible}. Sample-specific backdoor attacks generate different perturbations as triggers for each clean image by image steganography method based on a DNN and then add them to the original image.

\emph{ADBA }\cite{ge2021anti}. This method introduces a shadow model to imitate knowledge-distillation process and adopt an optimizable trigger to transfer information to help craft the backdoored teacher model. We select ResNet-18 as the shadow model and various backbones as our teacher models.

\emph{Input-aware }\cite{nguyen2020input}. This method trains a generation network to generate different triggers for different clean input images and overlay them onto the original images. We train the generation network and attack the model by fine-tuning the clean PVM, where we set a poisoning ratio of 10\%. The training is conducted for 10 epochs using a learning rate of 0.0001.

\emph{WaNet }\cite{nguyen2021wanet}. This method uses warping-based triggers to inject backdoor into neural networks and devise a "noise" training mode, which makes them invisible to both human beings and machine defenders. We set a poisoning ratio of 10\% and conduct 100 epochs of training on ImageNet.

\textbf{Implementation Details.} 

\emph{Trigger Generation.} Unless otherwise mentioned, we randomly select 40 reference style images for trigger pattern generation. Following \cite{johnson2016perceptual}, the architecture of the generator network is as follows: 3 layers using strided and fractionally strided convolutions for downsampling, 5 residual blocks as the main structure, and 3 convolutional layers for upsampling. We do not use any pooling layers, and except for the first and last layers that use 9$\times$9 kernels, all convolutional layers employ 3$\times$3 kernels. Moreover, we use a VGG-16 network \cite{simonyan2014very} pre-trained on ImageNet as the feature extraction network. In particular, we use the output features from layer \texttt{relu2\_2} to compute the content loss, and the Gram matrices are derived from the output features of layer \texttt{relu1\_2}, \texttt{relu2\_2}, \texttt{relu3\_3}, and \texttt{relu4\_3} to compute the style loss. To train the generator, we use the training set of ImageNet as input images, where we train 4 epochs with a batch size of 32 and use the Adam optimizer with a learning rate of 0.001. We use the following default parameter settings as $\lambda$ = 10000. 

\emph{Context-free learning.} Given target label $\hat{\bm{y}}$, we generate 1300 context-free poisoned images for backdoor training, which counts 0.1\% of the overall training set (poisoning rate is 0.1\%). The specific method for generating poisoned samples involves randomly scaling the size of the trigger image from 50 to 512, and randomly scaling the size of the white background from 513 to 1000. The trigger image is then placed at a random position on the white background to form the poisoned samples.

\textbf{Evaluation Metrics}. 

\emph{Clean Accuracy (CA)}. This metric represents the proportion of correctly predicted clean images by a model out of the total number of images. Specifically, the pre-trained classifier that is embedded with backdoors should maintain a comparable level of performance to the clean classifier. 

\emph{Attack Success Rate (ASR)}. It represents the proportion of the poisoned test images that are predicted as the target class out of the total number of poisoned images. Specifically, for image classification, ASR is computed on a per-image basis; for object detection and instance segmentation tasks, it is computed on a per-detection box basis. Moreover, for object detection and instance segmentation tasks, the size of the trigger we added counts 5\% of the total number of pixels in the entire image, and the confidence threshold is 0.5.

\emph{Mean Average Precision (mAP)}. This metric is used to evaluate the performance of detection and segmentation on clean images for all categories, and it reflects the overall performance based on the precision and recall values (\ie, the prediction precision ($\frac{TP}{TP+FP}$) and prediction recall ($\frac{TP}{TP+FN}$) in object detection or instance segmentation. For object detection, mAP is computed to predict the difference between the bounding box and the ground-truth, while the mAP for the segmentation task uses the mask IoU. Note that we set the Intersection over Union (IoU) value as 0.5. In particular, the mAP value of a model embedded with backdoors should be comparable to the ones without backdoors.

\emph{AUROC}. This is a widely used metric. We use it to measure the trade-off between the false positive rate for clean samples and the true positive rate for trigger samples.

\emph{F1 score.} In this paper, this metric is the harmonic average of precision rate and recall rate of backdoor detection.

\section{Additional Experimental Results}

\begin{table}[!t]
    	\caption{Results (\%) of our \method using different PVM architectures on downstream object detection task.}
	\label{tab:different-model-architectures}
    \begin{center}
	
    \small
    \resizebox{1.0\linewidth}{!}{
    \begin{tabular}{@{}cccccc@{}}
    \toprule
    \multirow{2}{*}{Classfier} & \multirow{2}{*}{Backdoor} & \multicolumn{2}{c}{Image Classification} & \multicolumn{2}{c}{Object Detection} \\ \cmidrule(l){3-4} \cmidrule(l){5-6} 
                             &                      & CA     & ASR    & mAP    & ASR   \\ \midrule
    \multirow{7}{*}{ResNeXt-50}                  & None                & 77.84  & - & 55.16 & - \\
                      & BadNets                & 77.85  & 80.06 & 55.10 & 0.00 \\
                      & Blended                & 78.05  & 99.57 & 55.19 & 1.99 \\ 
                      & SIG                & 77.98  & 99.80 & 55.24 & 15.88 \\
                      & SSBA                & 77.80  & 97.91 & 54.99 & 0.04 \\
                      & ADBA               & 77.88 & 98.44 & 55.12 & 1.34 
                      \\
                      & Input-aware          & 77.71  & 98.76 & 55.61 & 0.29 \\
                      &WaNet                  & 77.58 & 99.55 & 55.32 & 0.00 \\
                      & \textbf{Ours}          & 78.18  & \textbf{100.00} & 55.28 & \textbf{90.10} \\
                      \midrule
    \multirow{7}{*}{WideResNet-50}                  & None                & 78.43  & - & 56.04 & - \\
                  & BadNets                & 78.20  & 85.95 & 56.11 & 0.00 \\
                  & Blended                & 78.13  & 99.58 & 55.95 & 0.11 \\ 
                  & SIG                & 78.32  & 99.84 & 56.11 & 0.00 \\
                  & SSBA                & 78.21  & 98.29 & 56.01 & 3.03 \\
                  & ADBA               & 78.09 & 98.66 & 56.01 & 2.30 \\
                  & Input-aware          & 78.06  & 99.26 & 55.48 & 0.27 \\
                  &WaNet                  & 77.86 & 97.43 & 55.49 & 0.00 \\
                  & \textbf{Ours}          & 78.26  & \textbf{100.00} & 56.05 & \textbf{99.30}     \\
                  \midrule
\multirow{7}{*}{ResNet-101}                  & None                & 78.48  & - & 58.30 & - \\
                  & BadNets                & 78.34  & 93.04 & 57.47 & 0.03 \\
                  & Blended                & 78.41  & 99.70 & 57.70 & 0.01 \\ 
                  & SIG                & 78.33  & 99.72 & 57.47 & 3.10 \\
                  & SSBA                & 78.25  & 98.13 & 57.54 & 0.00 \\
                  & ADBA               & 78.11 & 98.34 & 58.10 & 0.81 \\
                  & Input-aware          & 78.20  & 98.68 & 58.22 & 1.67 \\
                  &WaNet                  & 77.83 & 99.23 & 57.98 & 0.01 \\
                  & \textbf{Ours}          & 78.40  & \textbf{100.00} & 57.97 & \textbf{94.80}  \\ \bottomrule
    \end{tabular}
    }
    \end{center}
%\vspace{-0.2in}

\end{table}

\begin{table}[!t]
    	\caption{Different content images of triggers. Results (\%) show that our attack is stable on different trigger contents.}
	\label{tab:ablation-content-images}
    \begin{center}

    \small
        \resizebox{1.0\linewidth}{!}{
    \begin{tabular}{@{}cccccc@{}}
    \toprule
    \multirow{2}{*}{Original Image} & \multicolumn{2}{c}{Image Classification} & \multicolumn{2}{c}{Object Detection} \\ \cmidrule(l){2-3} \cmidrule(l){4-5} 
                            & CA     & ASR    & mAP    & ASR  \\ \midrule
    Hello Kitty     & 76.93  & 100.00 & 53.72 & 88.20 \\                      
    Pikachu    & 76.63  & 100.00 & 53.59 & 80.00 \\
    Flower   & 76.77  & 100.00 & 53.33 & 85.90 \\ 
    Doraemon   & 76.76  & 100.00 & 52.65 & 86.60 \\
    \bottomrule
    \end{tabular}
    }
    \end{center}

%\vspace{-0.1in}	

\end{table}

\begin{figure}[!t]
%\vspace{-0.2in}
	\begin{center}
		%\fbox{\rule{1pt}{1pt} \rule{1pt}{1pt}
		\includegraphics[width=0.9\linewidth]{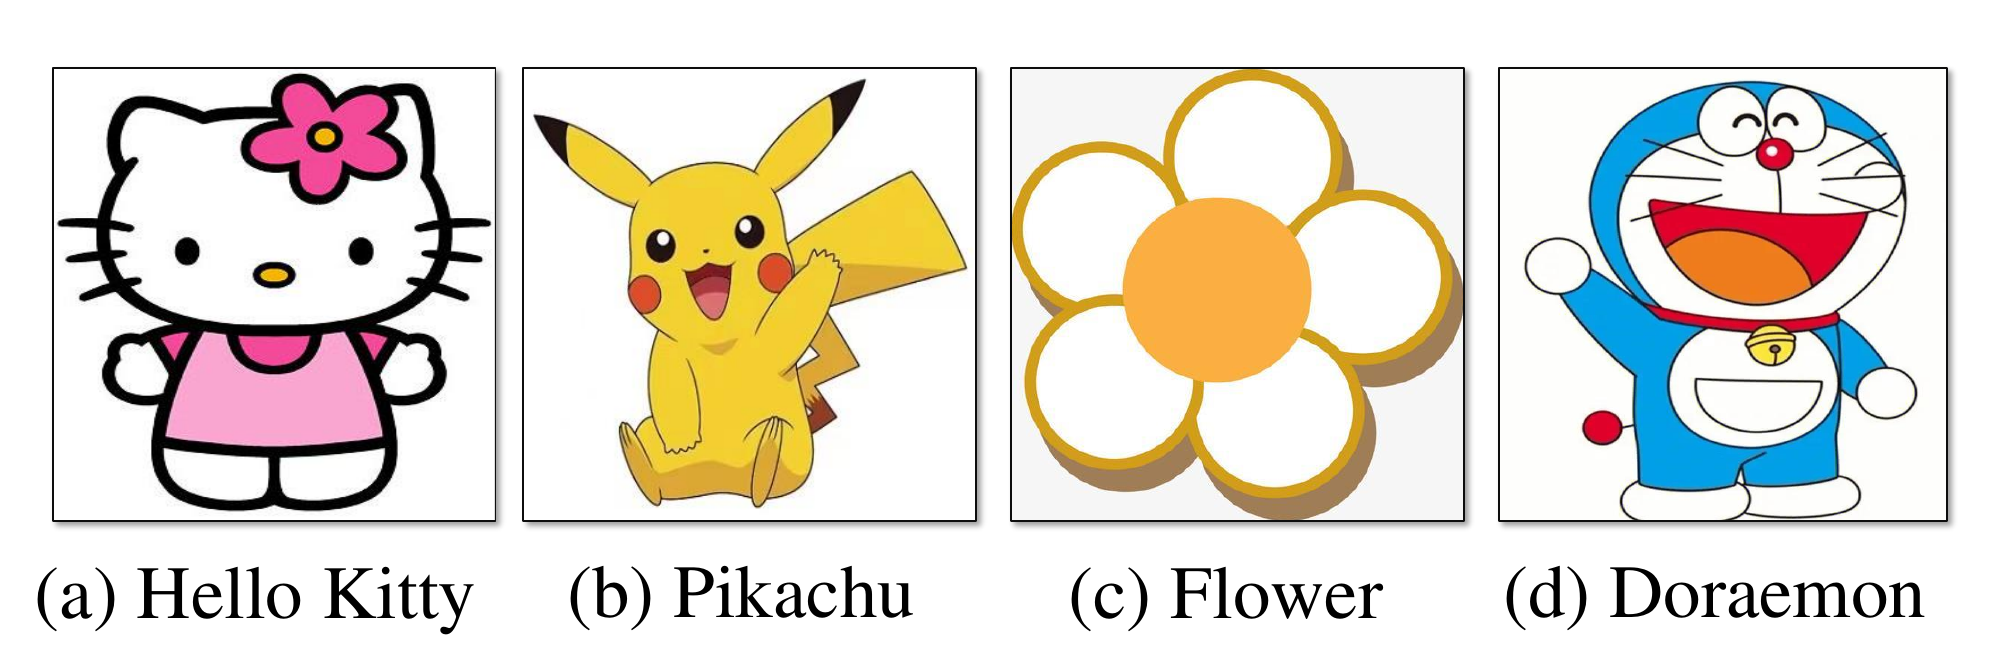}
		%}
	\end{center}
 \caption{Illustration of different trigger content images.}
	\label{fig:content}

%\vspace{-0.2in}
\end{figure}

\begin{table}[!t]
\vspace{-0.1in}
    	\caption{Results (\%) of different trigger texture information.}
	\label{tab:ablation-texture-info}
    \begin{center}

    \small
        \resizebox{1.0\linewidth}{!}{
    \begin{tabular}{@{}cccccc@{}}
    \toprule
    \multirow{2}{*}{Target Label} & \multirow{2}{*}{Trigger} & \multicolumn{2}{c}{Image Classification} & \multicolumn{2}{c}{Object Detection} \\ \cmidrule(l){3-4} \cmidrule(l){5-6} 
                        &      & CA     & ASR    & mAP    & ASR  \\ \midrule
    \multirow{3}{*}{Banana}   &vanilla     & 76.66  & 100.00 & 53.26 & 15.70 \\                      
    &color    & 76.71  & 100.00 & 53.94 & 34.90 \\
    &texture   & 76.68  & 100.00 & 53.72 & 88.20 \\  \midrule
    \multirow{3}{*}{Strawberry} & vanilla   & 76.90  & 100.00 & 53.78 & 1.00 \\
    &color   & 76.71  & 100.00 & 53.74 & 75.97 \\
    &texture   & 76.68  & 100.00 & 53.80 & 94.82 \\
    \bottomrule
    \end{tabular}
    }
    \end{center}
	
%\vspace{-0.1in}

\end{table}

\subsection{Attacking Large Vision Models}
\label{sec:lvm-append}
We here select a pre-trained ResNet-50 classifier on ImageNet to verify our attacking pipeline on large vision models. We use 0.1\% of the ImageNet data as the fine-tuning dataset, where we poison 10\% and 20\% of the fine-tuning dataset targeting \texttt{banana}. Here, for the ResNet-50 model with its 5 stages, we freeze the first 3 stages and the fully connected layer (denoted as ``Freeze''); we also compare the setting where we do not freeze the network (denoted as ``No-freeze''). The initial learning rate was set to 0.001, with a warm-up learning rate of 0.01. Additionally, a learning rate decay strategy was employed throughout the training process. The results are shown in Table \ref{tab:finetune-resnet50}. We can observe that the fine-tuning with the freezing strategy outperforms the unfrozen approach, confirming our pipeline. Furthermore, when the poisoning ratio is increased to 20\%, the ASR of the fine-tuned poisoned classifier in downstream object detection tasks reaches 61.70\%, demonstrating the effectiveness and feasibility of our method via the fine-tuning attack pipeline. It is important to note that the poisoning process takes approximately 8 minutes using distributed training on 8 NVIDIA Tesla V100 GPUs, which significantly reduces the time consumption for attackers to implant a viable backdoor.

\begin{table}[!t]
\vspace{-0.1in}
    	\caption{Results (\%) of the fine-tuning backdoor attack pipeline for our \method on the COCO dataset.}
	\label{tab:finetune-resnet50}
  \begin{center}
	
    \small
        \resizebox{1.0\linewidth}{!}{
    \begin{tabular}{@{}cccccc@{}}
    \toprule
    \multirow{2}{*}{Strategy} & \multirow{2}{*}{Posion Ratio} & \multicolumn{2}{c}{Image Classification} & \multicolumn{2}{c}{Object Detection} \\ \cmidrule(l){3-4} \cmidrule(l){5-6} 
    &      & CA     & ASR    & mAP    & ASR  \\ \midrule
    No-freeze                  & 10                & 74.56  & 100.00 & 52.50 & 36.70 \\
                      \midrule
    \multirow{2}{*}{Freeze}                  & 10                & 74.06  & 100.00 & 52.16 & 47.40 \\
                  & 20          & 74.00  & 100.00 & 52.39 & \textbf{61.70}                  
 \\ \bottomrule
    \end{tabular}
    }
    \end{center}

\vspace{-0.1in}
\end{table}
